# Supplementary material for: Aspects of entanglement with background electric and magnetic fields in quantum field theoretic systems
Source: arXiv:2311.01014 source file (2023-11-02)
Supplement: Supplementary file 1 [file appendix.tex]

\appendixname{A}
